# Supplementary material for: Interpretability Guarantees with Merlin-Arthur Classifiers
Source: arXiv:2206.00759 source file (2024-03-22)
Supplement: Supplementary file 2 [file param_69_fig.tex]

\documentclass[10cm]{standalone}
\usepackage[utf8]{inputenc}
\usepackage{tikz, pgfplots}
\pgfplotsset{compat=1.15}
\usepackage{array,multirow,booktabs}

\input{abbrv}

\begin{document}

\Large{
\centering
\begin{tabular}{@{}c@{\hspace{-0.2em}}c@{\;}c@{\hspace{1.2cm}}m{0.6cm}}
%%%%%%%%%%%%%%%%%%%%%%%%%%%%%%%%%%%%%%%%%%%%
& Hybrid & \hspace{1em} Network  \\
%%%%%%%%%%%%%%%%%%%%%%%%%%%%%%%%%%%%%%%%%%%%
&
\raisebox{-.5\height}{\includegraphics[height=4cm]{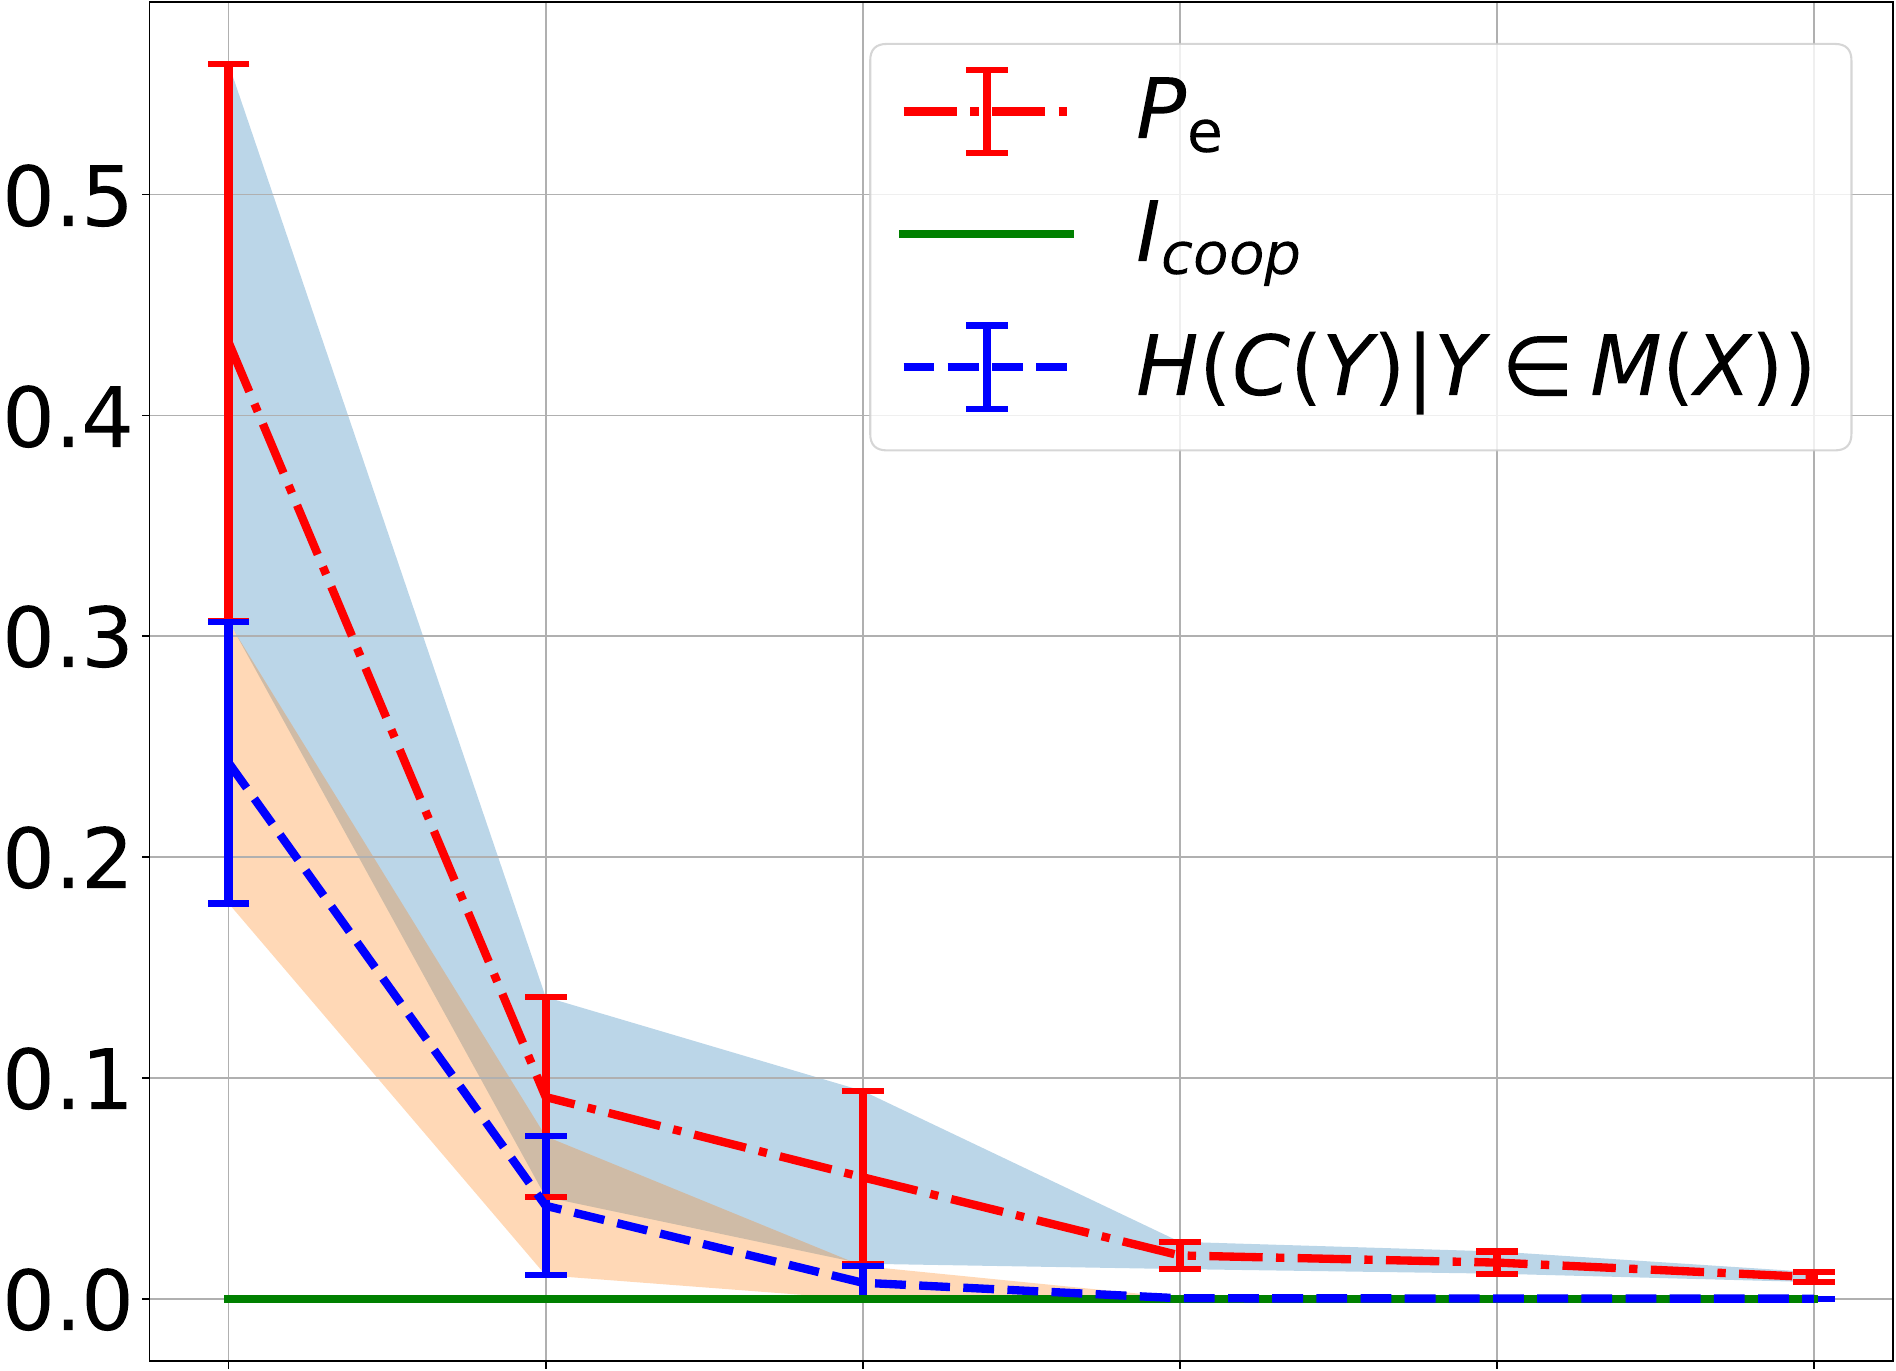}}
&
\raisebox{-.5\height}{\includegraphics[height=4cm]{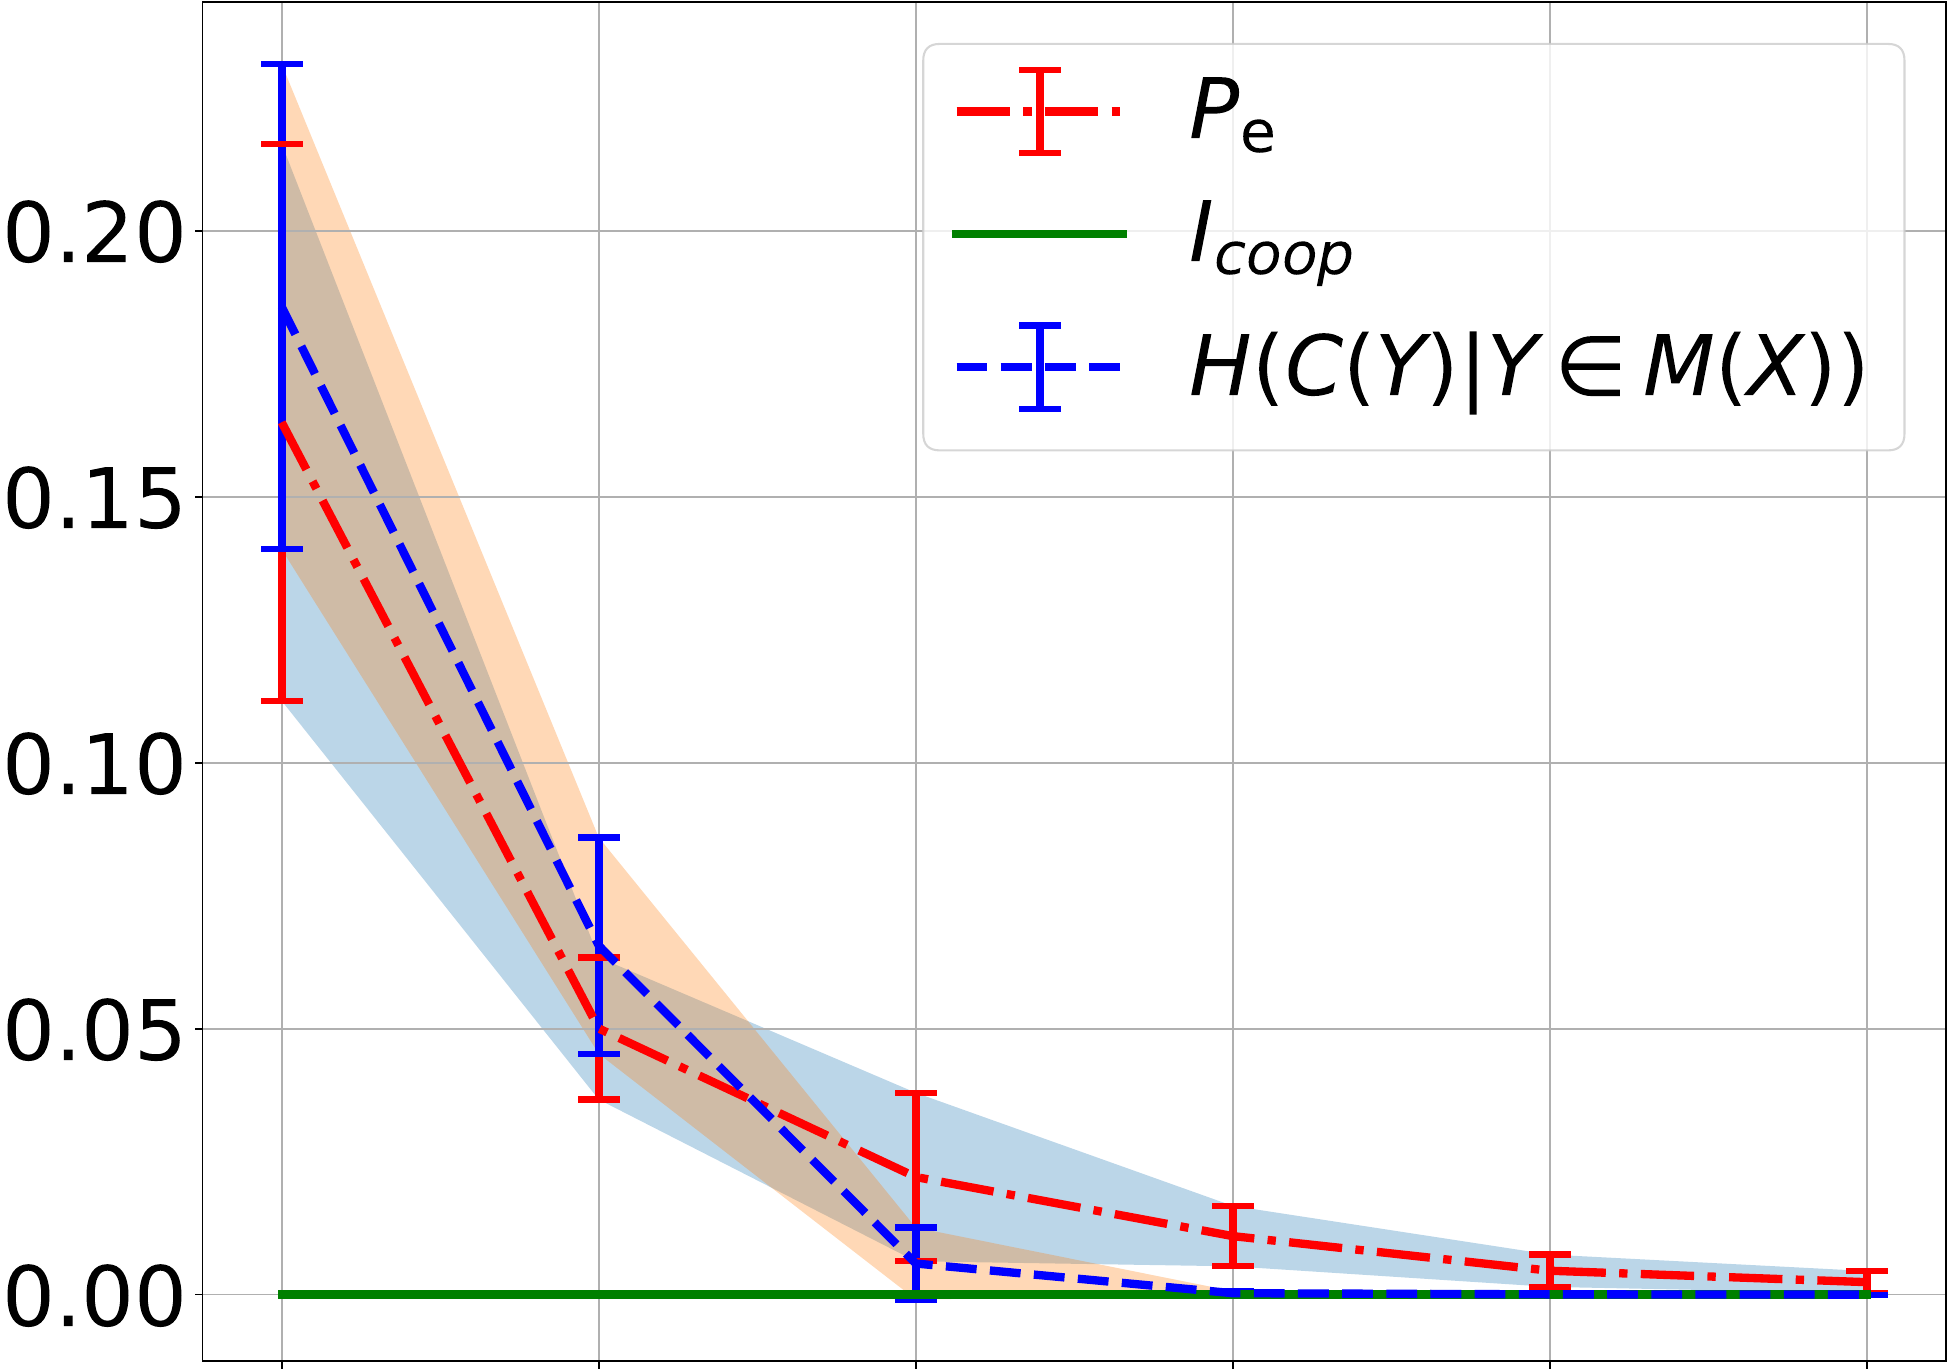}}
\\
%%%%%%%%%%%%%%%%%%%%%%%%%%%%%%%%%%%%%%%%%%%%
&
\hspace{1em}\includegraphics[width=5cm]{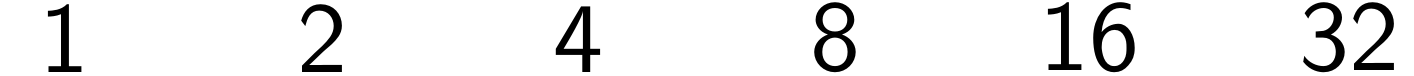}
&
\hspace{1em}\includegraphics[width=5cm]{img/fano_violation/fano_x_scale.pdf}
\\
%%%%%%%%%%%%%%%%%%%%%%%%%%%%%%%%%%%%%%%%%%%%
&
$k$
&
$k$

%%%%%%%%%%%%%%%%%%%%%%%%%%%%%%%%%%%%%%%%%%%%
\end{tabular}
}
\end{document}
